# Supplementary material for: Revisiting the flocking transition using active spins
Source: arXiv:1303.4427 ancillary file (2013-09-06)
Supplement: Supplementary file 1 [file Supplements.pdf]

# Supplementary Information—Revisiting the flocking transition using active spins

A. P. Solon[1], J. Tailleur[1]

[1] *Univ Paris Diderot, Sorbonne Paris Cite, MSC, UMR 7057 CNRS, F75205 Paris, France*

(Dated: July 21, 2013)

PACS numbers: 87.18.Gh, 05.65.+b, 45.70.Vn

## CONSISTENCY OF THE MEAN-FIELD APPROXIMATION IN THE LIMIT $\rho \to \infty$

Beyond the assumptions leading to the RMFM ($m \ll \rho$ and $\beta_c = 1+\frac{r}{\rho}$), we used another aproximation to compute the profiles exactly (Eqs. (MT-7) and (MT-8) of the main text (MT)): we neglected the $\tilde{D}\Delta\rho$ term in Eq.(MT-1) and linearized the density around $\rho = \rho_1$ to obtain Eq. (MT-6). These two approximations are self-consistent in the limit $T \to 1$ and/or $\rho_0 \to \infty$.

Indeed, $\tilde{D}\Delta\rho \sim \tilde{D}\frac{(\rho_h-\rho_\ell)}{l_i^2}$ where $l_i$ is the size of the interface which scales like $1/q$, so that $\tilde{D}\Delta\rho \sim q^2 \sim 1/\rho_1^2$ which has to be compared to $v\partial_x m \sim m_h/l_i \sim q \sim 1/\rho_1$. This can also be checked directly by computing these two terms using the exact solution shown in the main text.

Then, when rewriting the density $\rho = \rho_1(1+\delta\rho)$, $\delta\rho$ becomes smaller and smaller as $T \to 1$. Indeed, $\rho_h - \rho_\ell$ remains constant while $\rho_1$ diverges in this limit, so that the relative difference between $\rho$ and $\rho_1$ vanishes when $T \simeq 1$. This justifies the two aforementioned approximations as well as the $m \ll \rho$ approximation.

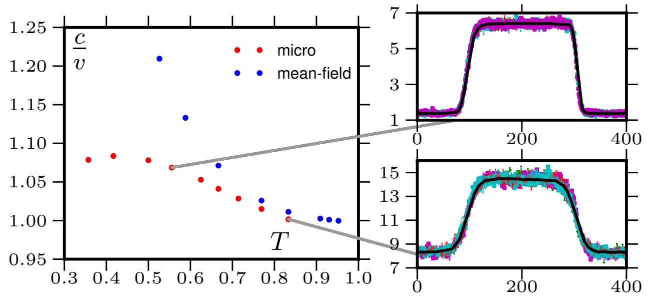


FIG. 1. **Left**: relative speed $c/v$ of the traveling bands compared to the velocity of individuals in the 2d microscopic model (red) and simulations of the RMFM (blue). For the microscopic model, points are obtained by tracking the bands after averaging over the transverse direction. **Right**: superposition of density profiles averaged in the transverse direction for two temperatures showing the relative importance of fluctuations and time-averaged profile (black thick curve). Linear size $L = 400$, $D = 1$, $\varepsilon = 0.9$, $v = 1.8$, $r = 1$.

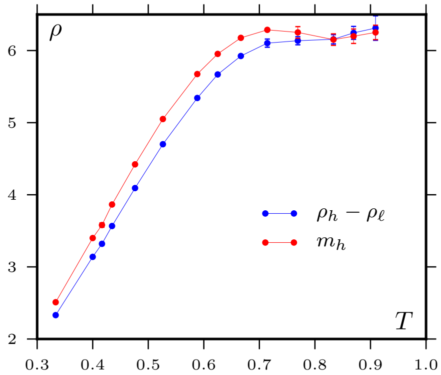


FIG. 2. $\rho_h - \rho_\ell$ (blue) and $m_h$ (red) in the 2d microscopic model, ($\rho_h$,$m_h$) being the density and magnetization in the liquid phase and $\rho_\ell$ the density in the gas phase. Error bars increase as $T \to 1$ due to fluctuations that become larger (see fig. 1 right). $D = 1$, $\varepsilon = 0.9$.

## NUMERICAL CHECKS OF THE RMFM PREDICTIONS

The results predicted by the refined mean-field model (RMFM) cannot be tested for arbitrarily large $\rho$, first due to computational limitations and then because the time-averaging process becomes more and more difficult as the density increases. To average profiles over time we indeed need to find the frame comoving with the liquid phase and thus to detect the position of the fronts. Fluctuations make it difficult so that we first average the profiles in the transverse direction. As $T$ gets closer to 1, the density increases and so do the density fluctuations (see fig. 1 right) so that we need to use larger and larger systems to average out part of the fluctuations. Ultimately, fluctuations of the position of the front in the longitudinal direction comes into play and smoothen artificially the averaged profile so that we are not able to compute the underlying front anymore. At lower densities, we do not encounter this problem and time-averaging the density profile is much easier. Finally, this averaging problem is critical for the front profile but much less when measuring the values of $\rho_h$ and $\rho_\ell$ which can thus be computed for larger densities.

Even though we cannot reach arbitrarily large densities, which restrains the temperature range accessible numerically, our results suffice to check the theoretical predictions of the RMFM in the limit $\rho \to \infty$.

First, we find that as $T$ tends to 1, $\rho_h - \rho_\ell = m_h$ tends to a constant (see fig. 2).

| $\rho_0$ | $\phi$ | $c$ |
|---|---|---|
| 2.8 | 0.285 | 1.923 |
| 4 | 0.525 | 1.924 |
| 5.3 | 0.785 | 1.924 |

TABLE I. Speed of the liquid phase for different average densities $\rho_0$ at constant temperature. Changing $\rho_0$ only changes the fraction of liquid $\phi$ (defined using a threshold at half of the liquid/gas interface) but not $c$. The error is estimated to be $\Delta c = 2.10^{-3}$ from the variability of $c$ on different data sets for the same parameters. $T = 0.55$, $D = 1$, $\varepsilon = 0.9$, linear size $L = 400$.

Then, as $T \to 1$ the velocity of the liquid bands $c$ gets closer and closer to its putative asymptotic value $v = 2D\varepsilon$, the velocity of the individual particles (see fig. 1 left). $c$ can be larger than $v$ since in addition to the drift velocity $v$ there is a FKPP-like velocity [6] steming from the "reactions" between $+$ and $-$ spins at the front of the band. (Note that the "analogy" is between the density in the FKPP equation and the magnetization here. The "creation" of ordered sites at the front of the band is only possible because the disordered gas phase has a non-zero density.) The intake and loss of "birds" in the flock can thus make the flock propagates faster than the individual birds. Note that we have checked that the same holds for the Vicsek model where the band can propagate faster than $\langle v_{\parallel} \rangle$ (the average of the component of the order parameter pointing in the direction in which the band propagates). There, however, since $\langle v_{\parallel} \rangle < v$, one often has $\langle v_{\parallel} \rangle < c < v$ [7]. Such effect should actually be quite generic for systems in which the liquid phase propagates in a non-zero density background and it would be interesting to know if it could be measured experimentally, for instance for vibrated polar disks [2] or assemblies of locusts [1].

Also, for a given temperature, the speed $c$ does not depend on the average density $\rho_0$ that only controls the fraction of liquid $\phi$ as can be seen in table I showing $c(\rho_0)$ for $T = 0.55$.

Finally, one can compare the density profiles obtained in simulations of the microscopic model and of the RMFM. When $\beta$ gets closer to 1, the profiles become more and more symmetric and can be fitted with the analytical form Eq.(MT-7), as shown in Fig. 4. For lower temperature, the term $\tilde{D}\Delta\rho$ in Eq. (MT-1) cannot be neglected. This term is responsible for the asymmetry of the fronts as can be seen by writing the RMFM equations in the frame comoving with a liquid band:

$$0 = \tilde{D}\Delta\rho + c\partial_x\rho - v\partial_x m \tag{1}$$

$$0 = \tilde{D}\Delta m + c\partial_x m - v\partial_x\rho + 2m(\beta - 1 - \frac{r}{\rho}) - \alpha\frac{m^3}{\rho^2} \tag{2}$$

Integrating Eq.(1) over space one gets

$$\tilde{D}\partial_x\rho + c\rho - vm = cte = c\rho_\ell \tag{3}$$

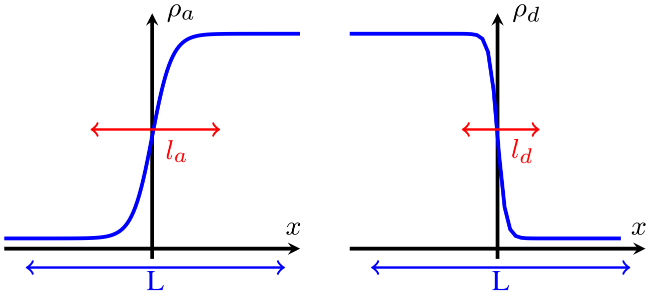


FIG. 3. Ascending and descending front solution of equations (1)-(2).

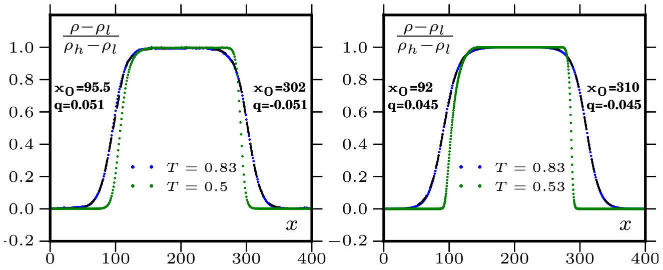


FIG. 4. Rescaled density profiles in the 2d microscopic model (left) and RMFM (right) at low temperature (green) and higher temperature (blue). As temperature is increased, profiles become more symmetric and the fronts can eventually be fitted by the analytical forms $\frac{\rho-\rho_\ell}{\rho_h-\rho_\ell} = \frac{1}{2}(1 \pm \tanh[q(x - x_0)])$ (black dashed line) with $q$ and $x_0$ the fitting parameters. On the contrary, at low temperature, the asymmetric profiles cannot be fitted with this form. $D = 1$, $\varepsilon = 0.9$, $L = 400$ for the microscopic model. $r = v = D = 1$, $L = 400$ for the RMFM.

Let us call $\rho_{a/d}(x)$, $m_{a/d}(x)$ the profiles corresponding to ascending and descending fronts, respectively (see figure 3). Integrating Eq. (3) along a domain of length $L$ much larger than the front widths $l_{a/d}$, one obtains

$$\tilde{D}(\rho_h - \rho_\ell) + \int_{-L/2}^{L/2} dx(c\rho_a - vm_a) = c\rho_\ell L \tag{4}$$

$$\tilde{D}(\rho_\ell - \rho_h) + \int_{-L/2}^{L/2} dx(c\rho_d - vm_d) = c\rho_\ell L \tag{5}$$

Substracting Eqs. (4) and (5) we arrive at

$$2\tilde{D}(\rho_h - \rho_\ell) + c\Big[\int_{-L/2}^{L/2} dx(\rho_a - \rho_d)\Big] - v\Big[\int_{-L/2}^{L/2} dx(m_a - m_d)\Big] = 0 \tag{6}$$

For symmetric fronts, $\rho_a(x) = \rho_d(-x)$, $m_a(x) = m_d(-x)$, and we are left $2\tilde{D}(\rho_h - \rho_\ell) = 0$, so that symmetric fronts are only possible if the diffusive term $\tilde{D}\Delta\rho$ can be neglected in Eq. (MT-1).

## DENSITY-DEPENDENCE IN THE RMFM

The dependence of the spinodal line with density $\beta_c = 1 + \frac{r}{\rho}$ can be seen as the first term of a Taylor expansion $\beta_c(\rho) = 1 + \sum_{n>0} \frac{r_n}{\rho^n}$ which suggests that $\beta_c$ is an analytic function of $1/\rho$ in the neighborhood of $1/\rho = 0$. A similar strategy was for instance used in the context of Bose-Einstein condensation to estimate corrections to the critical temperature due to the finiteness of the number of atoms in a condensate [8].

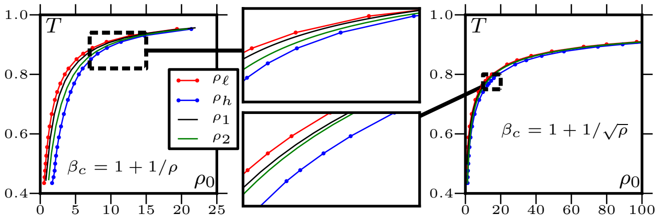


FIG. 5. Comparison of the phase diagrams of the RMFM with a $1/\rho$ dependence of $\beta_c(\rho)$ (left) and $1/\sqrt{\rho}$ dependence (right). $v = 1, r = 1$

In principle, we could have used a more general expansion $\beta_c = 1 + \sum_{n\geq 0} \frac{r_n}{\rho^{n\nu}}$ with $\nu > 0$ an arbitrary real number. Such a choice does not change the phase diagram or density profiles qualitatively, which shows that the RMFM predictions are quite robust with respect to the details of $\beta_c(\rho)$. Indeed, since our expansion of the RMFM Eq.[MT-5,6] is a linearization around $\rho = \rho_1$, changing the functional form $\beta_c(\rho)$ only changes constants in the results Eq.[MT-8]. Then, Fig. 5 shows the phase diagrams for a $1/\rho$ and a $1/\sqrt{\rho}$ dependence and we see that the diagram is indeed altered quantitatively but not qualitatively.

In microscopic simulations, we typically see 'activated events' leading to phase-separated profiles before the spinodal line is reached so that $\nu$ and $r$ cannot be directly computed from microscopic simulations. Since their precise values do not affect qualitatively the predictions of the RMFM, we used the simpler $1/\rho$ corrections in our simulations. Note that since mean-field typically overestimate the critical temperature by neglecting collective fluctuations, we chose $r > 0$ in all our study.

Last, note that it would in principle be possible for the coexistence lines to merge at a finite density from which a line of continuous transitions would lead to $\rho = \infty$. This is however not supported by Fig. 2 which shows $\rho_h - \rho_\ell$ to tend to a non-vanishing constant as $T$ goes to 1, preventing the merging of these lines for finite densities.

## NUMBER FLUCTUATIONS

In their phenomenologic theory of flocking [3], Toner and Tu predicted that the homogeneous ordered phase should exhibit giant density fluctuations. These can be

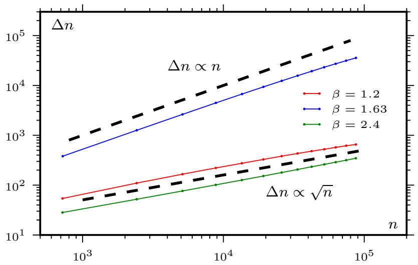


FIG. 6. Number fluctuations in the 2d microscopic model for the three different phases: gas (red), liquid (green) and coexistence (blue). $n$ is the number of particles in boxes of size $\ell$ and $\Delta n$ its root mean square. $D = 1$, $\varepsilon = 0.9$, $L = 400$, $\rho_0 = 5$

measured by looking at the fluctuations in the number $n$ of particles in a box of size $\ell$ and computing the corresponding root mean square $\Delta n$. Even though giant number fluctuations—when $\Delta n \sim n^\mu$ with $\mu > 1/2$—are difficult to measure precisely, their occurrence has been reported in a number of studies, for example in the Vicsek model [4] where $\mu \approx 0.8$. In particular, a reason why such fluctuations are difficult to measure is that they can easily be mistaken for the density fluctuations arising from standard phase-separation (and conversely) which yields $\mu = 1$ [5].

In our model, where homogeneous and phase-separated profiles are easy to discriminate, we measure normal Gaussian number fluctuations, $\mu = 1/2$, in the ordered liquid as well as in the gas phase (see fig. 6). We thus only see giant fluctuations with $\mu = 1$ in the coexistence region which are trivially attributed to phase-separation and no sign of the anomalous fluctuations $\mu \simeq 0.8$ traditionnaly associated to flocking states.

In the Toner and Tu phenomenological theory, giant number fluctuations are paired with the superdiffusion in the direction transverse to the direction of motion. This superdiffusion is typically associated with the fluctuations of the particles velocities in the direction transverse to the propagation of the flock. In our model, however, we have scalar order parameter and velocities with discrete symmetries, and thus normal diffusion in the direction transverse to the propagation of the flock. This may explain why we do not see giant number fluctuations. All in all, this shows that a polar flocking state can exist without giant number fluctuations and calls for an even greater care when measuring number fluctuations in flocking models.


[1] J. Buhl, D. J. T. Sumpter, I. D. Couzin, J. J. Hale, E. Despland, E. R. Miller, S. J. Simpson, *Science* **312**, 1402 (2006)

[2] J. Deseigne, O. Dauchot, and H. Chat, *Phys. Rev. Lett/* **105**, 098001 (2010); C. A. Weber, and T. Hanke, J. Deseigne, S. Léonard, O. Dauchot, E. Frey, H. Chaté, *Phys. Rev. Lett.* **110**, 208001 (2013)

[3] J. Toner and Y. Tu, Phys. Rev. Lett. **75**, 4326 (1995); Phys. Rev. E **58**, 4828 (1998); J. Toner, Phys. Rev. Lett. **108**, 088102 (2012); Phys.Rev.E **86**, 031918 (2012)

[4] G. Grégoire, H. Chaté, Phys. Rev. Lett. **92** 025702 (2004); H. Chaté, F. Ginelli, G. Grégoire, F. Raynaud, Phys. Rev. E **77** 046113 (2008).

[5] I. S. Aranson *et al.*, Science **320** 612 (2008)

[6] R. A. Fisher. Ann. Eugenics **7**:353369, 1937

[7] A. Solon *et al.*, in preparation.

[8] W. Ketterle, N. J. Van Druten, Phys. Rev. A **54**, 656 (1996)
